# Supplementary material for: Tiny Sc allows the chains to rattle: Impact of Lu and Y doping on the charge density wave in ScV$_6$Sn$_6$
Source: arXiv:2306.07868 ancillary file (2023-06-13)
Supplement: Supplementary file 1 [file Lu_Y_Doped_ScV6Sn6_SI_01.pdf]

# Sc allows the chains to rattle: Impact of Lu and Y doping on the charge density wave in $ScV_6Sn_6$

# Supplemental Information

William R. Meier,[*,†] Richa Pokharel Madhogaria,[†] Shirin Mozaffari,[†] Madalynn Marshall,[‡] David E. Graf,[¶] Michael A. McGuire,[§] Hasitha W. Suriya Arachchige,[‖] Caleb L. Allen,[‖] Jeremy Driver,[‖] Huibo Cao,[‡] and David Mandrus[*,‖]

†*Materials Science & Engineering Department, University of Tennessee Knoxville, Knoxville, Tennessee 37996, USA*

‡*Neutron Scattering Division, Oak Ridge National Laboratory, Oak Ridge, Tennessee 37831, USA*

¶*National High Magnetic Field Laboratory, Tallahassee, FL, 32310, USA*

§*Material Science & Technology Division, Oak Ridge National Laboratory, Oak Ridge, Tennessee 37831, USA*

‖*Department of Physics & Astronomy, University of Tennessee Knoxville, Knoxville, Tennessee 37996, USA*

⊥*Materials Science & Technology Division, Oak Ridge National Laboratory, Oak Ridge, Tennessee 37831, USA*

E-mail: javamocham@gmail.com; dmandrus@utk.edu

# X-ray diffraction

Table 1: Single crystal refinement of $LuV_6Sn_6$ and $YV_6Sn_6$ at room temperature.

| Chemical formula | $LuV_6Sn_6$ | $YV_6Sn_6$ |
|---|---|---|
| Formula wt. (g/molF.U.) | 1106.69 | 1192.75 |
| Crystal system | hexagonal | |
| Space group | $P6/mmm$ (191) | |
| Temperature (K) | 300 | |
| $a = b$ (Å) | 5.4995(3) | 5.5169(4) |
| $c$ (Å) | 9.1642(8) | 9.1780(10) |
| $V$ (Å$^3$) | 240.03(4) | 241.92(4) |
| $Z$ | 1 | 1 |
| Density calculated (g/cm$^3$) | 8.251 | 7.596 |
| Extinction coefficient | 0.045(2) | 0.0387(15) |
| $\theta$ range (°) | 2.222 - 33.475 | 2.219 - 33.059 |
| No. reflections; $R_{\text{int}}$ | 2596; 0.0625 | 2669; 0.0347 |
| No. independent reflections | 225 | 227 |
| No. parameters | 16 | 16 |
| $R_1$; $wR_2(I > 2\delta(I))$ | 0.0241; 0.0513 | 0.0158; 0.0375 |
| Goodness of fit | 1.228 | 1.207 |
| Diffraction peak and hole (e$^-$/Å$^3$) | 2.671 and -3.920 | 1.445 and -1.215 |

Table 2: Atomic positions in $LuV_6Sn_6$

| Atom | Wyckoff | x | y | z | occupancy | $U_{\text{eq}}$ (Å$^2$) |
|---|---|---|---|---|---|---|
| Lu1 | 1a | 0 | 0 | 0 | 1 | 0.0087(2) |
| Sn1 | 2e | 0 | 0 | 0.33114(5) | 1 | 0.0083(2) |
| Sn2 | 2d | $\frac{1}{3}$ | $\frac{2}{3}$ | $\frac{1}{2}$ | 1 | 0.0069(2) |
| Sn3 | 2c | $\frac{1}{3}$ | $\frac{2}{3}$ | 0 | 1 | 0.0063(2) |
| V1 | 6i | $\frac{1}{2}$ | 0 | 0.24781(7) | 1 | 0.0064(2) |

# References


(1) Arachchige, H. W. S.; Meier, W. R.; Marshall, M.; Matsuoka, T.; Xue, R.; McGuire, M. A.; Hermann, R. P.; Cao, H.; Mandrus, D. Charge Density Wave in Kagome Lattice Intermetallic $ScV_6Sn_6$. *Physical Review Letters* **2022**, *129*, 216402.

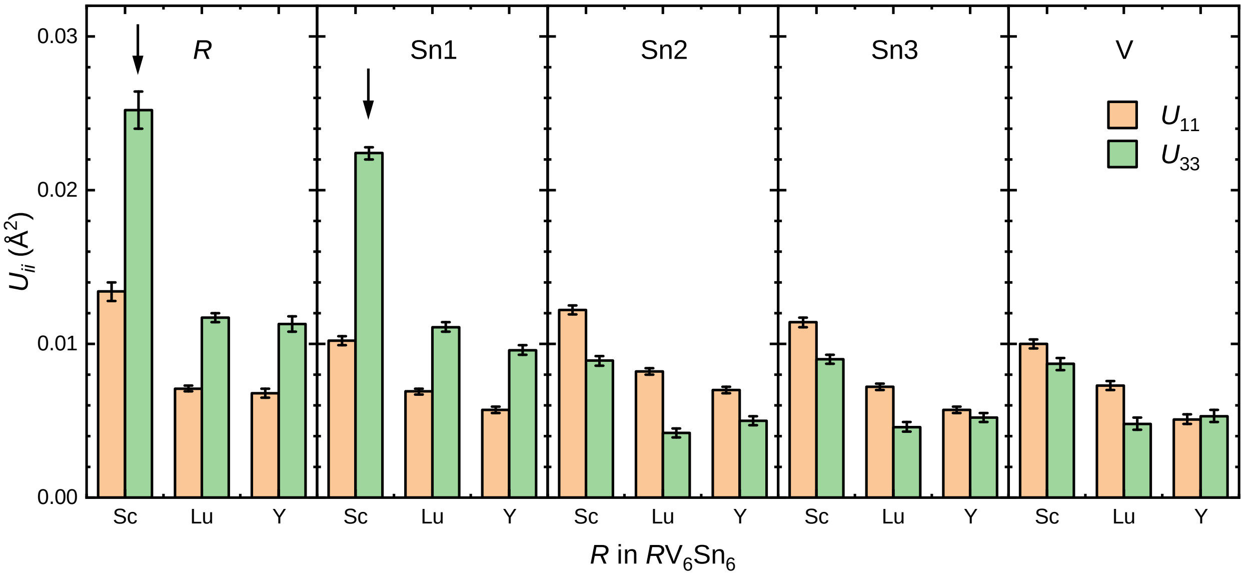


Figure 1: Room temperature anisotropic atomic displacement parameters (ADPs) for $R\mathrm{V_6Sn_6}$ compounds highlighting significantly larger $U_{33}$ values for the rare earth and Sn1 atoms in $\mathrm{ScV_6Sn_6}$ (arrows). The data for $\mathrm{ScV_6Sn_6}$ was taken from Arachchige et al.[1]

Table 3: Anisotropic displacement parameters for each atomic site of $\mathrm{LuV_6Sn_6}$

| Atom | $U_{11}$ (Å$^2$) | $U_{22}$ (Å$^2$) | $U_{33}$ (Å$^2$) | $U_{23}$ (Å$^2$) | $U_{13}$ (Å$^2$) | $U_{12}$ (Å$^2$) |
|---|---|---|---|---|---|---|
| Lu1 | 0.0071(2) | 0.0071(2) | 0.0117(3) | 0 | 0 | 0.00356(11) |
| Sn1 | 0.0069(2) | 0.0069(2) | 0.0111(3) | 0 | 0 | 0.00343(12) |
| Sn2 | 0.0082(2) | 0.0082(2) | 0.0042(3) | 0 | 0 | 0.00412(12) |
| Sn3 | 0.0072(2) | 0.0072(2) | 0.0046(3) | 0 | 0 | 0.00358(12) |
| V1 | 0.0073(3) | 0.0072(4) | 0.0048(4) | 0 | 0 | 0.0036(2) |

Table 4: Atomic positions in $\mathrm{YV_6Sn_6}$

| Atom | Wyckoff | x | y | z | occupancy | $U_{eq}$ (Å$^2$) |
|---|---|---|---|---|---|---|
| Y1 | 1a | 0 | 0 | 0 | 1 | 0.0083(2) |
| Sn1 | 2e | 0 | 0 | 0.33337(6) | 1 | 0.00702(17) |
| Sn2 | 2d | $\frac{1}{3}$ | $\frac{2}{3}$ | $\frac{1}{2}$ | 1 | 0.00635(16) |
| Sn3 | 2c | $\frac{1}{3}$ | $\frac{2}{3}$ | 0 | 1 | 0.00553(16) |
| V1 | 6i | $\frac{1}{2}$ | 0 | 0.24841(7) | 1 | 0.00528(19) |

Table 5: Anisotropic displacement parameters for each atomic site of $\mathrm{YV_6Sn_6}$

| Atom | $U_{11}$ (Å$^2$) | $U_{22}$ (Å$^2$) | $U_{33}$ (Å$^2$) | $U_{23}$ (Å$^2$) | $U_{13}$ (Å$^2$) | $U_{12}$ (Å$^2$) |
|---|---|---|---|---|---|---|
| Y1 | 0.0068(3) | 0.0068(3) | 0.0113(5) | 0 | 0 | 0.00342(16) |
| Sn1 | 0.0057(2) | 0.0057(2) | 0.0096(3) | 0 | 0 | 0.00287(10) |
| Sn2 | 0.0070(2) | 0.0070(2) | 0.0050(3) | 0 | 0 | 0.00351(10) |
| Sn3 | 0.0057(2) | 0.0057(2) | 0.0052(3) | 0 | 0 | 0.00285(10) |
| V1 | 0.0051(3) | 0.0055(4) | 0.0053(4) | 0 | 0 | 0.00274(19) |

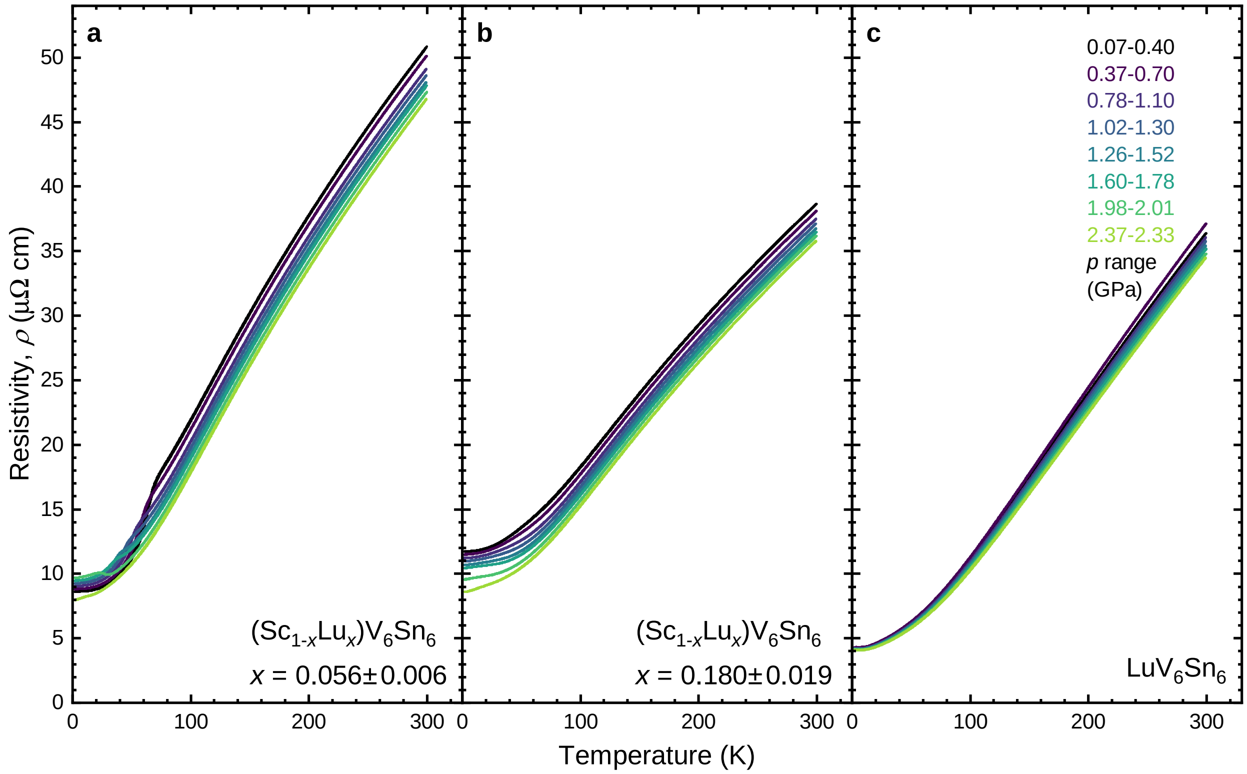


Figure 2: Evolution of resistivity vs temperature with increasing pressures for three $(Sc_{1-x}Lu_x)V_6Sn_6$ samples.

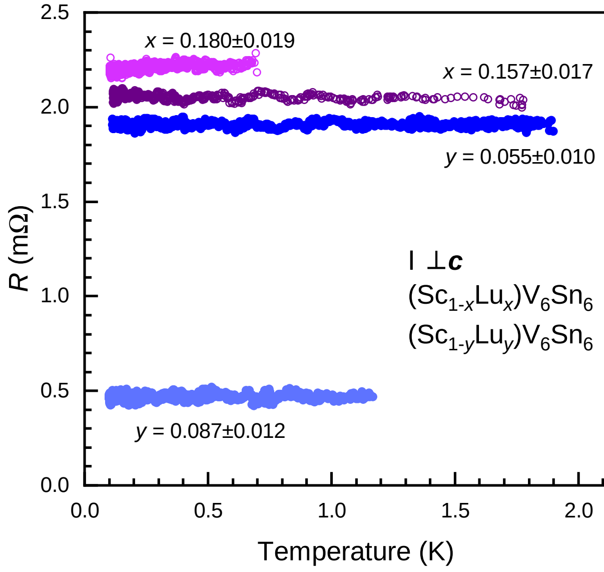


Figure 3: None of the Lu or Y doped $ScV_6Sn_6$ measured using the adiabatic demagnetization resistance setup show superconductivity.
